# Supplementary material for: New Feedback Control and Adaptive Evolve-Filter-Relax Regularization for the Navier-Stokes Equations in the Convection-Dominated Regime
Source: arXiv:2307.00675 source file (2025-07-10)
Supplement: Supplementary file 1 [file appendix_A.tex]

\section{The need of EFR and EFR-EFR need for uncontrolled Navier-Stokes}
\label{sec:uncontroled_example}
\subsection{{noEFR vs. EFR Numerical Comparison}}
\label{sec:exampleFOM}
In this section, we perform a numerical investigation of the role played by the EFR strategy in under-resolved \ms{marginally-resolved} FOM simulations.
To this end, we compare the following two approaches:
(i) noEFR, which is a standard numerical discretization of the NSE without an EFR regularization; and 
(ii) EFR, which is a standard numerical discretization of the NSE with an EFR regularization.
\ti{Are there other noEFR vs. EFR numerical comparisons?} \ms{Nope, I am planning to do that in the controlled setting}
\ti{I think it is more than a significant modification!  I'd say it is very different. I think we should say that we devised/constructed a new test problem to illustrate the pitfalls of using G-ROMs and G-FOM in the under-resolved regime. \ms{We now focus on the uncontrolled framework, which is extended to the feedback control setting in Section \ref{sec:problem}. We build a new test case that highlights the criticalities of the noEFR procedure in marginally-resolved regimes.}} 
We solve problem \eqref{eq:NSE}. The space domain is $\Omega \doteq \{[0, 2.2] \times [0, 0.41]\} \setminus \{(x, y)\in \mathbb R^2 \text{ such that } (x - 0.2)^2 + (y - 0.2)^2 - 0.05^2 = 0 \}$, represented in Figure \ref{fig:domain}. 
The Dirichlet boundary condition is 
\begin{equation}
\label{eq:inlet}
u_D = 
\begin{cases}
0 & \text{ on } \Gamma_W, \\
u_{\text{in}} = \displaystyle \left  ( \frac{6}{0.41^2}\sin(\pi t/8)y(0.41 - y), 0 \right) & \text{ on } \Gamma_{\text{in}}
\end{cases}
\end{equation}
where $\Gamma_W$ %is 
are the bottom ($\Gamma_B$) and the top ($\Gamma_T$) walls of the channel together with the walls of the cylinder ($\Gamma_C$) (solid teal boundary in Figure \ref{fig:domain}). The inlet condition $u_{\text{in}}$ is applied to $\Gamma_{\text{in}} = \{0\} \times [0, 0.41]$, (magenta dashed line in Figure \ref{fig:domain}). The prescribed inlet condition is given by equation \eqref{eq:inlet}.
Moreover, $\Gamma_N$ (black dotted boundary in Figure \ref{fig:domain}) features homogeneous Neumann conditions.
The initial condition is $u_0 = (0,0)$. The mesh parameters of the triangular mesh (depicted in Figure \ref{fig:mesh}) are:
 $h_{min} = 4.46 \cdot 10^{-3}$ and $h_{max} = 4.02 \cdot 10^{-2}$. After a Taylor-Hood $\mathbb P^2 - \mathbb P^1$ FE discretization for velocity and pressure, respectively, we obtain a FE space with $N_h \doteq N_h^{u} + N_h^p = 14053$ degrees of freedom. With this mesh parameters, as stated in \cite{Strazzullo20223148}, we are working in a marginally-resolved regime and for high values of $Re$, the simulation does not captures the features of the flow, presenting numerical oscillations.

\begin{figure}[H]
\centering
\hspace{-8mm}\includegraphics[scale=0.27]{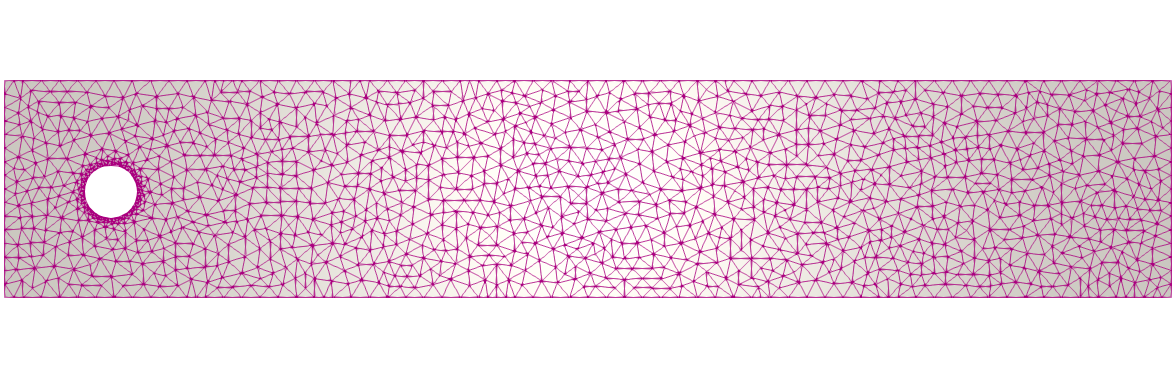}
\caption{{The mesh.}
}
\label{fig:mesh}
\end{figure}
\begin{figure}[H]
\begin{center}
\begin{tikzpicture}[scale=5.0]

\filldraw[color=teal!80, fill=gray!10, very thick](0.2,0.2) circle (0.05);
\filldraw[color=magenta!90, very thick, dashed](0,0) -- (0.,0.41);
\filldraw[color=teal!80, fill=gray!10, very thick](0,0.41) -- (2.2,0.41);
\filldraw[color=teal!80, fill=gray!10, very thick](0,0.) -- (2.2,0.);
\filldraw[color=black!80, fill=gray!10, very thick, dotted](2.2,0.) -- (2.2,0.41);

\node at (-.1,0.25){\color{black}{$\Gamma_{\text{in}}$}};
\node at (2.3,0.25){\color{black}{$\Gamma_{N}$}};
\node at (0,-.05){\color{black}{$(0,0)$}};
%\node at (3,-.3){\color{black}{$(1,0)$}};
%\node at (7.5,-.3){\color{black}{$(1 + \mu_2,0)$}};
%
\node at (0,0.45){\color{black}{$(0,0.41)$}};
\node at (2.35,0.45){\color{black}{$(2.2,0.41)$}};
\node at (2.3,-0.05){\color{black}{$(2.2,0)$}};
\node at (0.35,.2){\color{black}{$ \Gamma_C$}};
\node at (0.99,.45){\color{black}{$ \Gamma_T$}};
\node at (0.99,-.05){\color{black}{$ \Gamma_B$}};

\end{tikzpicture}
\end{center}
\caption{Schematic representation of the domain $\Omega$. $\gamma_D = \Gamma_{\text{in}} \cup \Gamma_C \cup \Gamma_T \cup \Gamma_B$. No-slip conditions are applied over the teal solid boundary. The inlet condition is applied to $\Gamma_{\text{in}}$, i.e. the magenta dashed line. $\Gamma_N$ (black dotted line) features Neumann boundary conditions.
}
\label{fig:domain}
\end{figure}

For example, this is the case when we set $\nu = 10^{-4}$ and $T=8 - \Delta t \sim 8$, for $\Delta t = 4\cdot 10^{-4}$. Differently from \cite{Strazzullo20223148}, where %they 
we work with $0 \leq Re \leq 100$, we are working with a %significantly larger 
Reynolds number that is { one order of magnitude higher}: $0 \leq Re \leq 1000$. 
%\ti{Emphasize this!  What $Re$ did we use in \cite{Strazzullo20223148}?} \ms{Done}
At the FOM level, the EFR algorithm was necessary to deal with this value of $Re$. Indeed, when no EFR algortihm was employed, the Newton's method used to solve the problem for each time instance diverged for $t \sim 4$. 
%Thus, 
{In contrast, the} EFR algorithm is able to alleviate the oscillations arising from convection-dominated problems and allows to reach a physical simulation. The differential filter radius is $\delta = 1.22\cdot 10^{-2}$ and $\chi = 5\cdot \Delta t$. The relaxation parameter is the one used in \cite{Strazzullo20223148}, the filter radius is chosen in the following way. We took the reference value of the filtered radius as in \cite{Strazzullo20223148}, say $ \hat{\delta}=(\sqrt{2})\delta^* $ with $\delta^* = 4.46\cdot 10^{-3}$ and %we choose 
chose $\delta$ as the minimum value in the set \todo{change the values, they are not correct, see code on the EFR-EFR folder} 
$\{\sqrt{2}\delta^*,\sqrt{2.25}\delta^*, \sqrt{2.5}\delta^*,\sqrt{2.75}\delta^*, \sqrt{3}\delta^*, \sqrt{3.25}\delta^*, \sqrt{3.5}\delta^*, \sqrt{3.75}\delta^*, \sqrt{4}\delta^*\}$ that guarantees the convergence of the Newton's solver. 
 Specifically, $\delta =\sqrt{3.5}\delta^*= 1.22\cdot 10^{-2}$. \ti{What is the principle used in choosing these values?} \ms{The parameters, where chosen with the idea of increasing the action of the differential filter over the domain. To do so, we increased the multiplicative value in front of $\delta^*$ with a trial-and-error approach}.\\ Choosing $\delta$ larger \ti{larger than what?} \ms{than $\hat{\delta}$} was needed in order to simulate the flow dynamics in the time interval $(0,8)$ with $Re=1000$. As already specified, if no EFR strategy is pursued offline, numerical instabilities propagate in time making the solution nonphysical and the Newton's solver %non-converging. 
{diverging}. This is shown in Figures \ref{fig:Netwon_v} and \ref{fig:Netwon_p}: they represent velocity and pressure fields for $t = 3.86, 3.9, 3.94$ for standard NS with noEFR (left plots) and EFR (right plots). The value $t=3.98$ is the one related to a diverging Newton's solver. In these plots we observe numerical oscillations around the cylinder that propagates going on in the time evolution. 
The phenomenon is also highlighted in Figure \ref{fig:blow-up}. Here, we observe a blow-up of the pressure norm, that is responsible of the numerical oscillations of Figure \ref{fig:Netwon_p}. The EFR strategy avoids the increase of energy of the pressure field and the simulation can be performed for the whole time interval $(0,8)$. We also observe that standard FE velocity $L^2-$norm coincides with the EFR velocity $L^2-$norm.
It is clear from the plot that a longer simulation in time would require a larger value of $\delta$, avoiding the propagation of the numerical instabilities in time.

\begin{figure}
        \centering \includegraphics[scale=0.25]{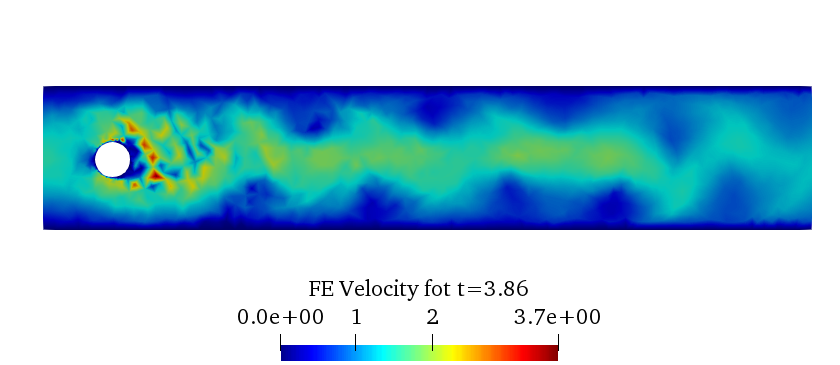}
        \centering  \includegraphics[scale=0.25]{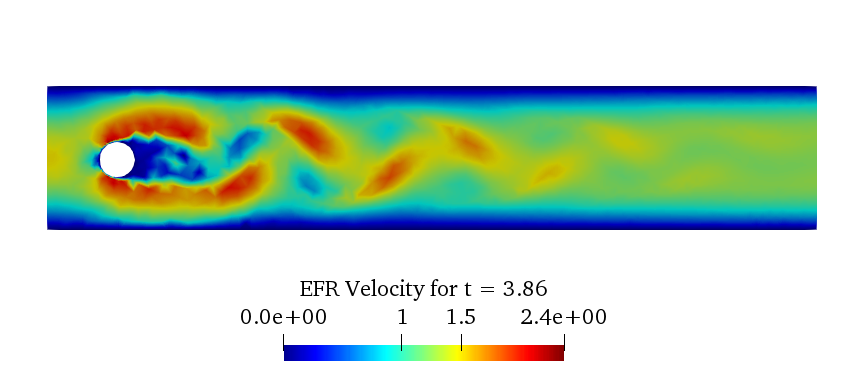}\\
        \centering \includegraphics[scale=0.25]{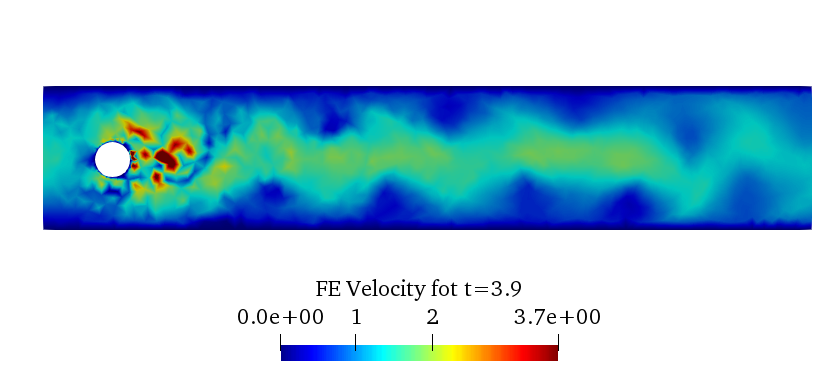}
        \centering \includegraphics[scale=0.25]{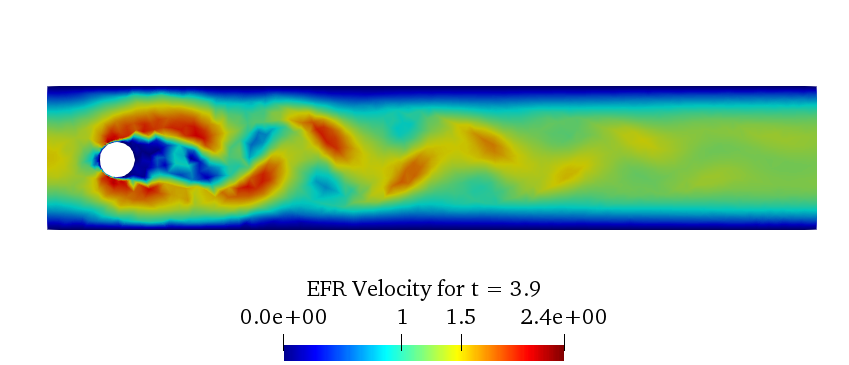}\\
        \centering \includegraphics[scale=0.25]{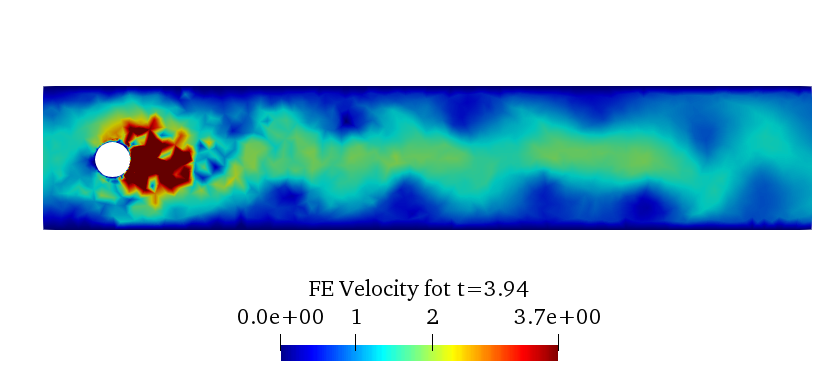}
        \centering \includegraphics[scale=0.25]{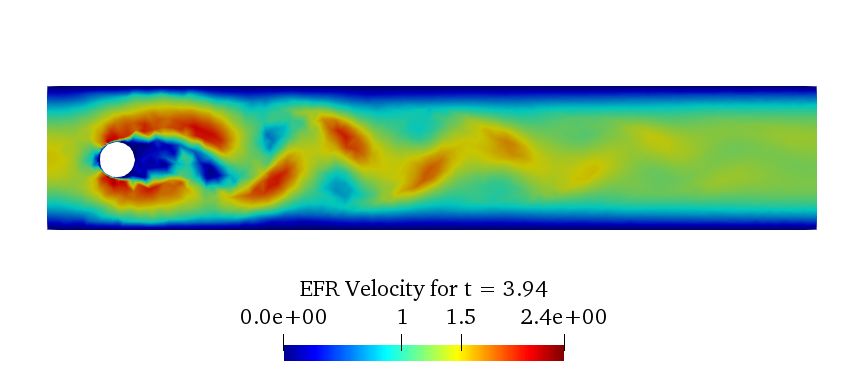}

\caption{\scriptsize{Representative FOM solutions for velocity: no-EFR (left plots) and EFR (right plots). From top to bottom: $t=3.86$, $t=3.9$, $t=3.94$.}
\label{fig:Netwon_v}
}\end{figure}

\begin{figure}[H]
        \centering \includegraphics[scale=0.25]{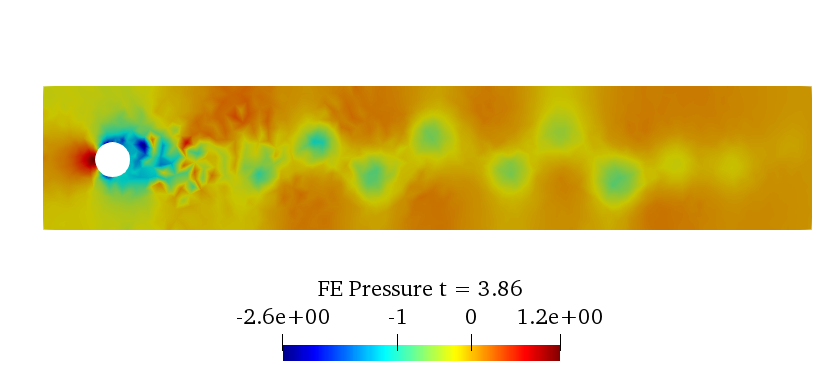}
        \centering 
        \includegraphics[scale=0.25]{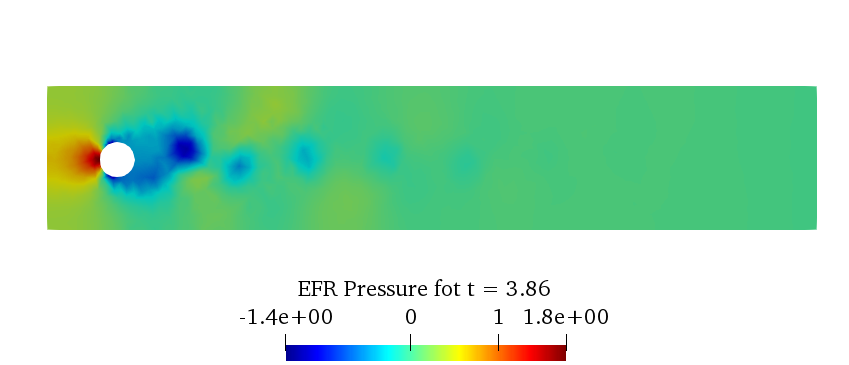}\\
        \centering \includegraphics[scale=0.25]{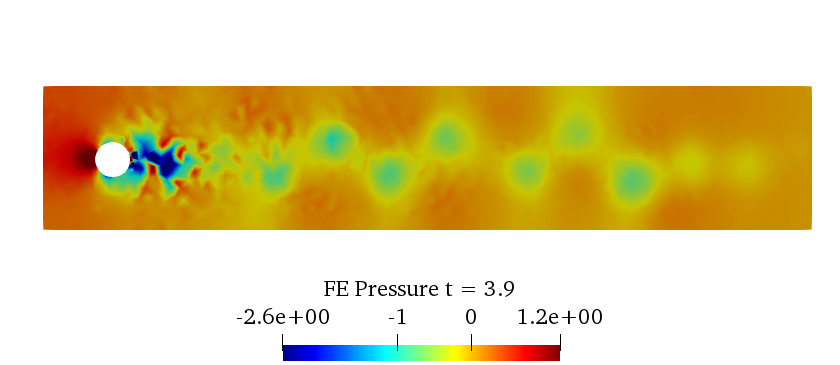}
        \centering \includegraphics[scale=0.25]{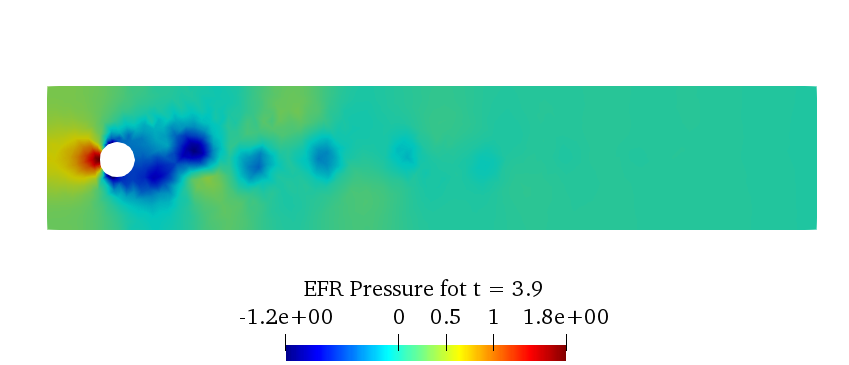}\\
        \centering \includegraphics[scale=0.25]{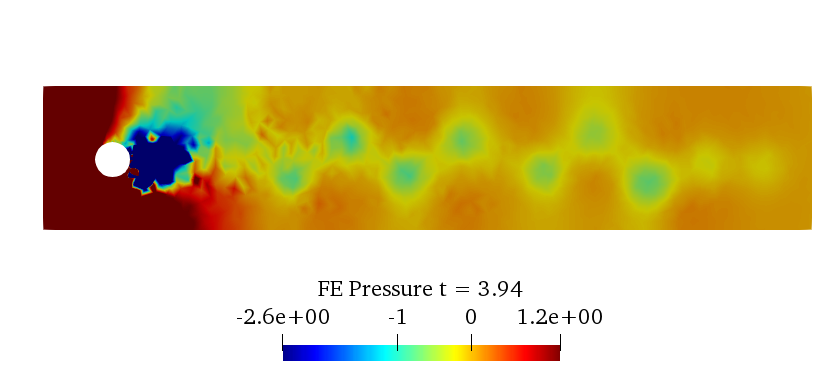}
        \centering \includegraphics[scale=0.25]{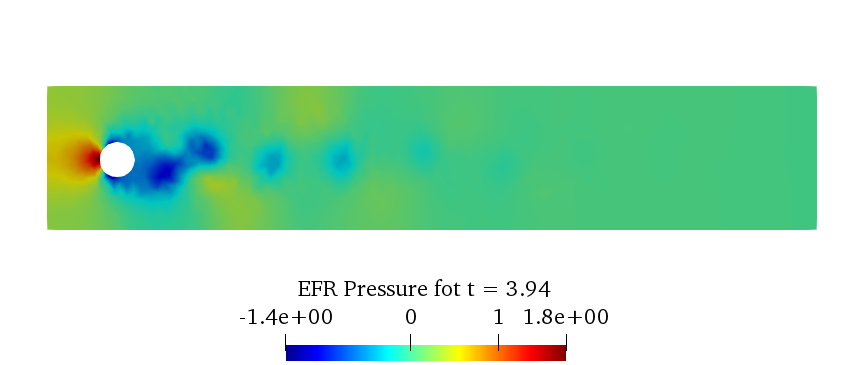}

\caption{\scriptsize{Representative FOM solutions for pressure: no-EFR (left plots) and EFR (right plots). From top to bottom: $t=3.86$, $t=3.9$, $t=3.94$.}
\label{fig:Netwon_p}
}\end{figure}

\begin{figure}
  \centering
  \includegraphics[width=0.49\textwidth]{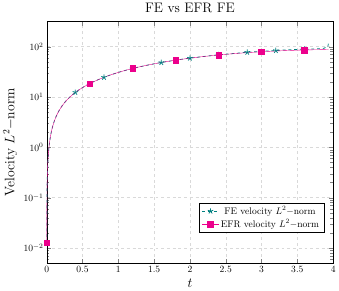}
  \includegraphics[width=0.49\textwidth]{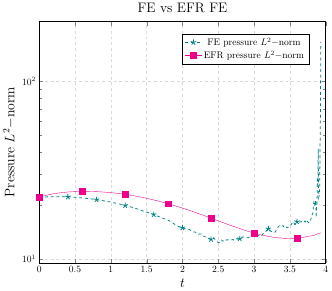}\\
   
  \caption{FE (teal dashed line) and EFR (magenta solid line) velocity and pressure $L^2-$norm in $(0, 3.94)$ for $\nu=10^{-4}, \delta=1.22\cdot 10^{-2}, \chi = 5\cdot \Delta t$, left and right plot, respectively}
  \label{fig:blow-up}
  \end{figure}

\subsection{{EFR-noEFR vs. EFR-EFR Numerical Comparison}}
In this section, we perform a numerical investigation of the role played by the EFR strategy in under-resolved ROM simulations.
To this end, we compare the following two approaches:
(i) EFR-noEFR, which is the standard G-ROM without an EFR regularization; and 
(ii) EFR-EFR, which is the standard G-ROM with an EFR regularization.
\ti{Are there other EFR-noEFR vs. EFR-EFR numerical comparisons?} \ms{no, there will be in the controlled setting}
The FOM setting is the EFR presented in section \ref{sec:exampleFOM}. \\ We recall the parameters used. The triangular mesh parameters are
 $h_{min} = 4.46 \cdot 10^{-3}$ and $h_{max} = 4.02 \cdot 10^{-2}$ and by means of a Taylor-Hood $\mathbb P^2 - \mathbb P^1$ FE discretization we have $N_h \doteq N_h^{u} + N_h^p = 14053$ degrees of freedom. Moreover, $\nu = 10^{-4}$ ($Re = 1000$), $T=8 - \Delta t \sim 8$, for $\Delta t = 4\cdot 10^{-4}$, $\delta = 1.22\cdot 10^{-2}$ and $\chi = 5\cdot \Delta t$.\\
 For the EFR-EFR algorithm, we followed the consistency strategy proposed in \cite{Strazzullo20223148} and these parameters are used both at the FOM and at the ROM level. We show representative solutions in Figure \ref{fig:comp_uncontrolled}. The left plot are the EFR, EFR-noEFR and EFR-EFR velocity profiles for $t=8$, from top to bottom. Analogously, the pressure fields for the different strategies are represented in the right column of Figure \ref{fig:comp_uncontrolled}. 
 
 Let us focus on the EFR-noEFR (center row of the plots) and EFR-EFR strategy (bottom row of the plots). For the reduction, we use $r_u=r_s=r_p=5$ obtained by a POD approach over 2000 equispaced snapshots in $(0,T)$. The number of used modes is limited, thus, we are working in a ROM under-resolved regime. We observe a better representation of the EFR velocity if we employ EFR algorithm at the ROM level, too. This complies with the conclusion of \cite{Strazzullo20223148}: EFR-EFR strategy is beneficial in terms of accuracy with respect to the EFR FOM simulation. Indeed, observing the EFR-noEFR velocity, we notice that the filtered and relaxed velocities have a maximum magnitude around \ti{change} \ms{$0.5$ while the EFR-noEFR strategy is beyond $1$}.
Moreover, for the velocity, some numerical oscillations arise just after the cylinder. This nonphysical behavior can be seen in the pressure field to, leading to an inaccurate representation of it around the cylinder. These oscillations are smoothed out by the EFR-EFR approach. 
\begin{figure}[H]
        \centering \includegraphics[scale=0.25]{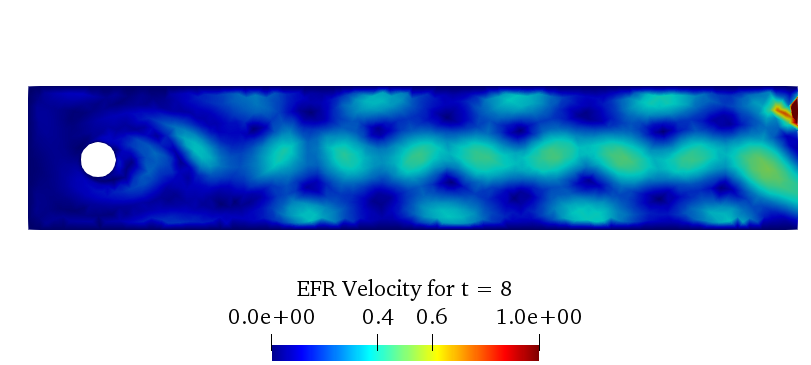}
        \centering \includegraphics[scale=0.25]{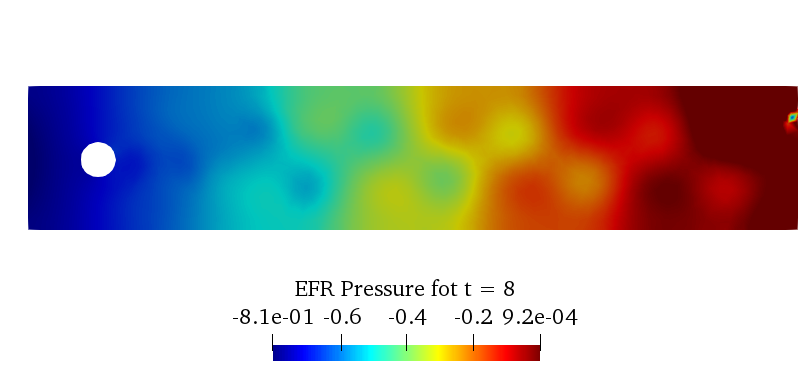}\\
        \centering \includegraphics[scale=0.25]{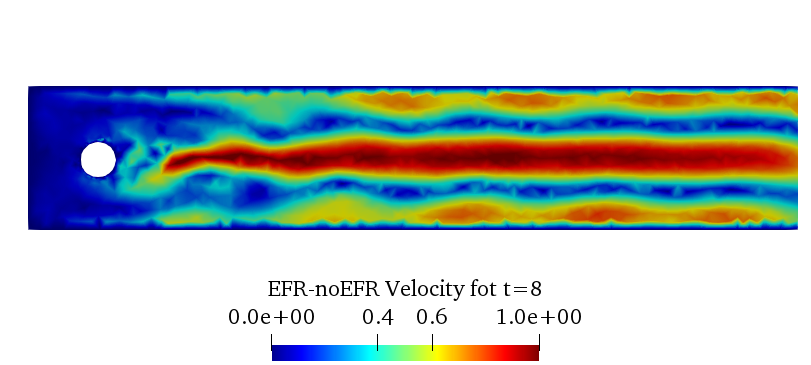}
        \centering \includegraphics[scale=0.25]{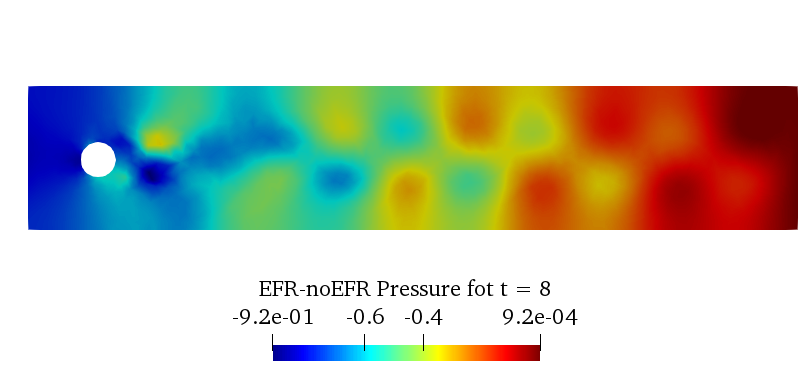}\\
        \centering \includegraphics[scale=0.25]{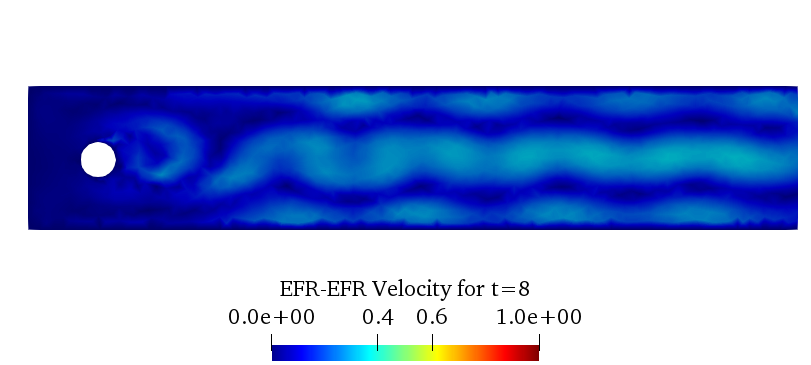}
        \centering \includegraphics[scale=0.25]{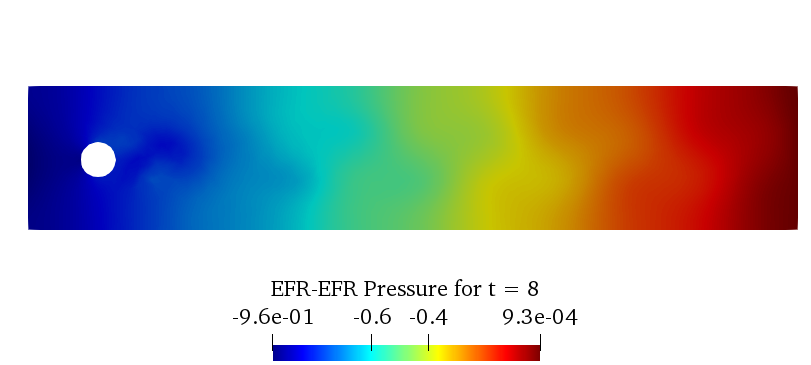}

\caption{{Representative solutions for velocity (left plots) and pressure (right plots) for $t=8-\Delta t, \nu=10^{-4}, \delta=1.22\cdot 10^{-2}, \chi = 5\cdot \Delta t, N_u=N_s=N_p=5$. From top to bottom: EFR FOM, EFR-noEFR, EFR-EFR.}
}
\label{fig:comp_uncontrolled}
\end{figure}
 
 These considerations are confirmed by Figure \ref{fig:plot_overline_uncontrolled}. We plot the velocity magnitude for the EFR, EFR-noEFR and EFR-EFR approaches over four segments: $\sigma_1 = \{2\} \times [0, 0.41], \sigma_2 = \{0.5\} \times [0, 0.41]$, $\sigma_3 = \{0.25\} \times [0.15, 0.25]$ and $\sigma_4 = [0.4, 2.2] \times \{0.205\}$. Namely, Figure \ref{fig:plot_overline_uncontrolled} analyzes the behavior of the flow:
\begin{itemize}
    \item[$\circ$] at the end of the channel on the $x_2$ axis with $\sigma_1$ (top left plot),
    \item[$\circ$] a bit after the cylinder on the $x_2$ axis with $\sigma_2$ (top right plot),
    \item[$\circ$] tangentially to the cylinder on the $x_2$ axis with $\sigma_3$ (bottom left plot),
    \item[$\circ$] longitudinally in the center of the domain on the $x_1$ axis, with $\sigma_4$ (bottom right plot).
\end{itemize}
The plots for $\sigma_1$ and $\sigma_2$ show that EFR-EFR is more accurate with respect to EFR-noEFR. Indeed, the reg-ROM is replicates the FOM bahavior for on $\sigma_1$. The compliance between the FOM solution and the EFR-EFR solution is less visible on $\sigma_2$.
\begin{figure}
  \centering
  \includegraphics[width=0.49\textwidth]{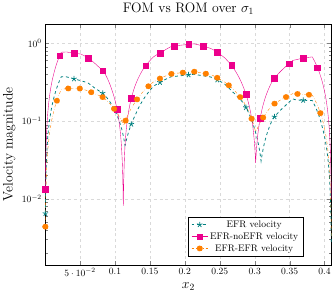}
  \includegraphics[width=0.49\textwidth]{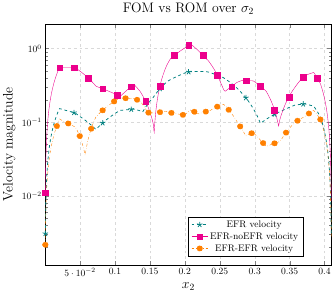}\\
   \includegraphics[width=0.49\textwidth]{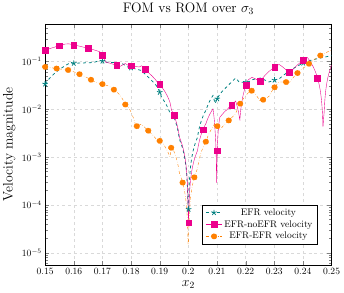}
      \includegraphics[width=0.49\textwidth]{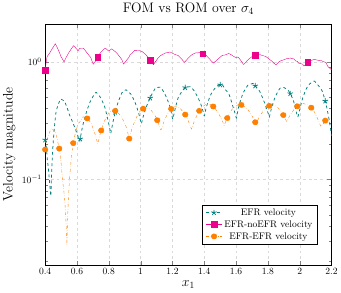}
  \caption{Velocity magnitude for $t=8-\Delta t, \nu=10^{-4}, \delta=1.22\cdot 10^{-2}, \chi = 5\cdot \Delta t, N_u=N_s=N_p=5$, over the segments $\sigma_1$ (top left plot), $\sigma_2$ (top right plot), $\sigma_3$ (bottom left plot), $\sigma_4$ (bottom right plot) for EFR (teal solid line), EFR-noEFR (magenta dashed line) and EFR-EFR (orange dashed-dotted line).}
  \label{fig:plot_overline_uncontrolled}
\end{figure}
However, the flow magnitude is comparable to the FOM one when it is close to the boundary. The drawback of using EFR-noEFR is clear in the bottom row of Figure \ref{fig:plot_overline_uncontrolled}. Indeed, on $\sigma_3$, EFR-noEFR is comparable to the FOM solution in the first half of the interval (i.e. lower part of the cylinder) while it oscillates in the second half of the interval (upper part of the cylinder). These oscillations are smoothed out by the EFR-EFR strategy, giving closer results to the FOM solution. The same can be observed along the the $x_1$ axis. The EFR-noEFR strategy is completely off in terms of magnitude and some numerical instabilities appear, most of all at the beginning of the interval. The EFR-EFR approach presents a smoother behavior and it is more accurate with respect to the EFR-noEFR strategy.

\begin{figure}[H]
  \centering
  \includegraphics[width=0.49\textwidth]{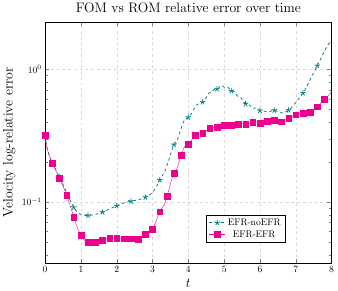}
  \includegraphics[width=0.49\textwidth]{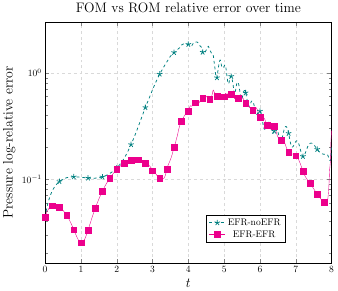}
  \caption{EFR-noEFR and EFR-EFR log-relative errors over time for $t=8-\Delta t, \nu=10^{-4}, \delta=1.22\cdot 10^{-2}, \chi = 5\cdot \Delta t, N_u=N_s=N_p=5$. The velocity and the pressure are represented in the left and right plot, respectively.}
  \label{fig:error_uncontrolled}
\end{figure}
The goal of this section is to justify the rational of the choice of the EFR-EFR strategy from now on. We observe that for a small %value 
{number} of modes,
\ti{I'd focus on stabilization instead of consistency.} \ms{another stabilization is beneficial and alleviates spurious numerical oscillations arising at the ROM level. This leads to better performances in terms of log-relative error for both velocity and pressure.} They are represented in Figure \ref{fig:error_uncontrolled}. Changing some parameters (online differential filter radius, online relaxation parameter, number of modes) can help increasing the accuracy even more but this is beyond the scope of this section. %From now on, 
{In what follows,} we employ the EFR-EFR approach. %The next section describes Navier-Stokes equation under a linear feedback control action.
