# Supplementary material for: New Feedback Control and Adaptive Evolve-Filter-Relax Regularization for the Navier-Stokes Equations in the Convection-Dominated Regime
Source: arXiv:2307.00675 source file (2025-07-10)
Supplement: Supplementary file 2 [file appendix_exp2.tex]

\section{Convergence results for time-dependent $U$}
\label{sec:exp2}
We propose a new numerical setting where the desired profile is $U + Ue^{-2t}$, where $U$ verifies \eqref{eq:Stokes}.

\begin{figure}[H]
  \centering
  \includegraphics[width=0.49\textwidth]{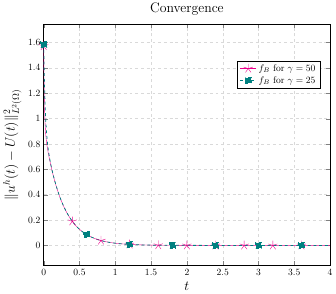}
  \includegraphics[width=0.49\textwidth]{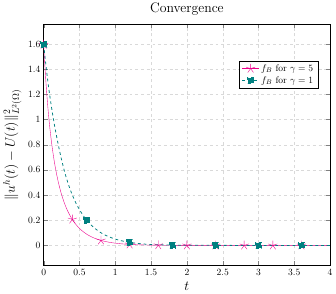}
  \caption{Experiment 2. Convergence results for $f_b$ for
  $\gamma \in \{50,25, 5, 1\}.$ For $\gamma=50, 25$ the approaches coincide. }
  \label{fig:exp2}
\end{figure}

\begin{figure}[H]
  \centering
  \includegraphics[width=0.49\textwidth]{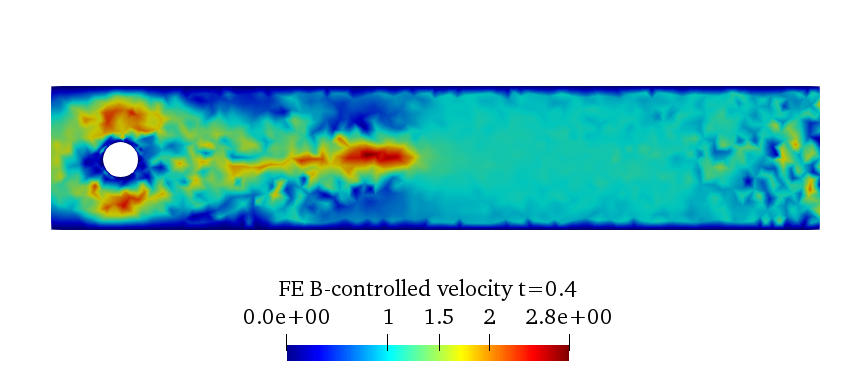}\\
  \includegraphics[width=0.49\textwidth]{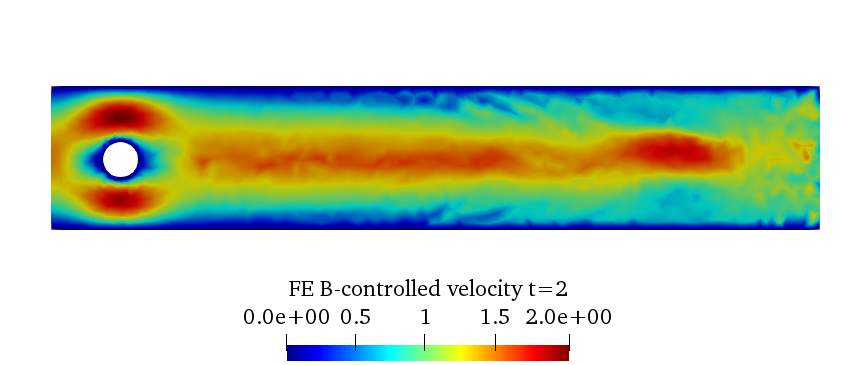}   \includegraphics[width=0.49\textwidth]{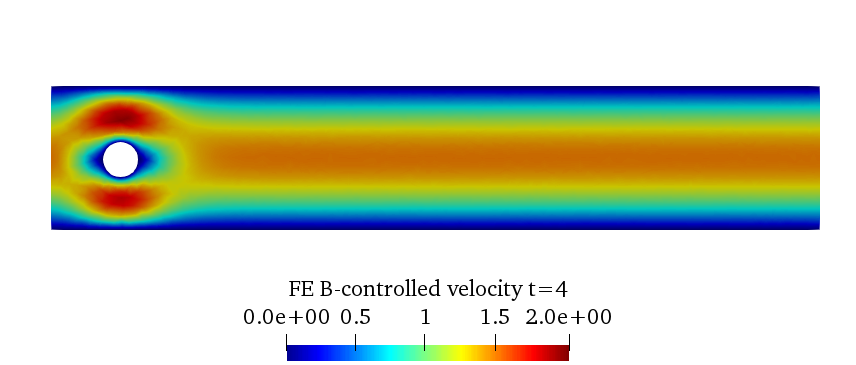}
  \caption{Experiment 1. B-controlled velocity for $t=0.4$ (top plot), $t=1.2$ (bottom left plot) and $t=4$ (bottom right plot) for $\gamma=10^{-4}$.}
  \label{fig:2solgamma0001}
\end{figure}

\begin{figure}[H]
  \centering
  \includegraphics[width=0.49\textwidth]{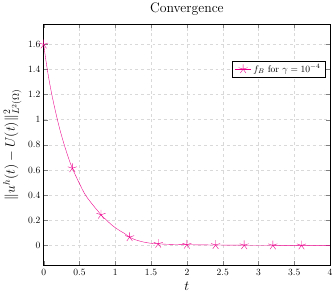}
  \includegraphics[width=0.49\textwidth]{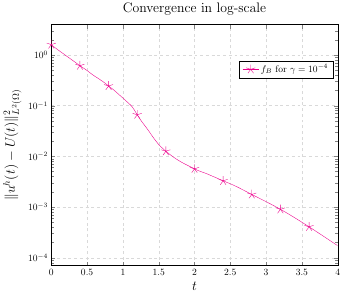}
  \caption{Experiment 2. Convergence results for $f_B$ for $\gamma=10^{-4}$. The left plot is proposed in log-scale on the right.}
  \label{fig:timeconvergencegamma0001}
\end{figure}
\todo{run EFR simulations and see if the convergence for $\gamma=10^{-4}$ is better}
\ms{Do you think we have to show Gunzburger's control? Or we stick with ours?}
\ms{with this example I have the exponential convergence! :D}

\ms{I discovered some new things:
\begin{itemize}
    \item we need to work with something that reaches a steady state (so no periodic BCs for the problem)
    \item the desired state $U$ must reach a steady state too (this is the reason why I am using $U + Ue^{-2t}$)
\end{itemize}
I hope to have some new results by tomorrow. The ones I had were not good for what we wanted to show. \\
I think that the setting we want to tackle is the one I am proposing here: steady BCs and unsteady $U(t) \rightarrow$ steady state (At least, I hope so).
\\ P.S. Gunzburger works with a time dependent problem, but it is almost stationary (the time derivative is almost null). This is the reason why they obtain very good convergence.
}

\ti{My understanding is that the goal of this section is to illustrate the need for EFR-EFR.  Is that correct?  I think we should clearly state the goals of each numerical experiment right from the start.}
